# Supplementary material for: Probabilistic semi-nonnegative matrix factorization: a Skellam-based framework
Source: arXiv:2107.03317 ancillary file (2021-07-07)
Supplement: Supplementary file 1 [file Skellam_snmf_supplementary_material.pdf]

# Skellam-SNMF: supplementary material

Benoit Fuentes

July 2, 2021

This document is the supplementary material attached to the paper *Probabilistic semi-nonnegative matrix factorization: a Skellam-based framework*. Prior reading of this article is essential to understanding this document. Section 1 is dedicated to the Skellam distribution and sections 2 and 3 to the detailed derivation of the EM and VBEM algorithms respectively.

## 1 Proofs about the Skellam distribution

**Definition 1** (Skellam random variable)**.** Let $\lambda_0, \lambda_1 \in \mathbb{R}^+$. If $X_0 \sim \mathrm{Pois}(\lambda_0)$ and $X_1 \sim \mathrm{Pois}(\lambda_1)$ are two independent Poisson r.v., then $X = X_0 - X_1$ is said to be distributed according to the Skellam distribution. One writes:

$$X \sim \mathrm{Skell}(\lambda_0, \lambda_1). \tag{1}$$

**Proposition 2** (Skellam distribution)**.** *If* $X_0 \sim \mathrm{Pois}(\lambda_0)$*,* $X_1 \sim \mathrm{Pois}(\lambda_1)$ *and* $X = X_0 - X_1 \sim \mathrm{Skell}(\lambda_0, \lambda_1)$*, then*

$$P(X = x) = \frac{{}_0F_1(|x|+1, \lambda_0\lambda_1)}{\Gamma(|x|+1)} \prod_{s\in\{0,1\}} e^{-\lambda_s} \lambda_s^{\max((-1)^s x, 0)} \tag{2}$$

*Proof.* Joint distribution of r.v. $X = X_0 - X_1$ and $Y = X_0 + X_1$ can be computed as:

$$\begin{aligned} P(X = x, Y = y) &= P\left(X_0 = \frac{y+x}{2}, X_1 = \frac{y-x}{2}\right) \\ &= P\left(X_0 = \frac{y+x}{2}\right) P\left(X_1 = \frac{y-x}{2}\right) \\ &= \frac{\lambda_0^{\frac{y+x}{2}} \lambda_1^{\frac{y-x}{2}}}{\frac{y+x}{2}!\,\frac{y-x}{2}!} e^{-(\lambda_0+\lambda_1)} \mathbb{1}_{y+x\equiv 0[2]} \mathbb{1}_{|x|\leq y}, \end{aligned}$$

$\mathbb{1}$ being the indicator function. Now, the distribution of $X$ is computed by marginalizing variable $Y$:

$$
\begin{aligned}
P(X=x) &= \sum_y P(X=x, Y=y \mid \lambda_0 \lambda_1) \\
&= e^{-(\lambda_0+\lambda_1)} \sum_y \frac{\lambda_0^{\frac{y+x}{2}} \lambda_1^{\frac{y-x}{2}}}{\frac{y+x}{2}!\,\frac{y-x}{2}!} \mathbb{1}_{y+x\equiv 0[2]} \mathbb{1}_{|x|\leq y} \\
&= e^{-(\lambda_0+\lambda_1)} \left(\frac{\lambda_0}{\lambda_1}\right)^{x/2} \sum_y \frac{(\lambda_0\lambda_1)^{\frac{y+|x|}{2}}}{\frac{y+|x|+x}{2}!\,\frac{y+|x|-x}{2}!} \mathbb{1}_{y\equiv 0[2]} \\
&= e^{-(\lambda_0+\lambda_1)} \left(\frac{\lambda_0}{\lambda_1}\right)^{x/2} \sum_y \frac{\left(\sqrt{\lambda_0\lambda_1}\right)^{2y+|x|}}{\Gamma(y+|x|+1)\,y!} \\
&= e^{-(\lambda_0+\lambda_1)} \left(\frac{\lambda_0}{\lambda_1}\right)^{x/2} \mathrm{I}_{|x|}\left(2\sqrt{\lambda_0\lambda_1}\right),
\end{aligned} \tag{3}
$$

$\mathrm{I}_v$ being the modified Bessel function of the first kind. Finally equation (2) is derived easily from equation (3) by formulating the relationship between $\mathrm{I}_v$ and ${}_0F_1$. □

**Proposition 3** (Stability by convolution of Skellam distribution)**.** *If $Z_n \sim \mathrm{Skell}(\lambda_{0,n}, \lambda_{1,n})$ for $n = 1 \ldots N$ are independent, then*

$$X = \sum_n Z_n \sim \mathrm{Skell}\left(\sum_n \lambda_{0,n}, \sum_n \lambda_{1,n}\right) \tag{4}$$

*Proof.* Each $Z_n$ is the difference between $Z_{0,n} \sim \mathrm{Pois}(\lambda_{0,n})$ and $Z_{1,n} \sim \mathrm{Pois}(\lambda_{1,n})$. $\sum_n Z_n = \sum_n Z_{0,n} - \sum_n Z_{1,n}$ with $\sum_n Z_{0,n} \sim \mathrm{Pois}(\sum_n \lambda_{0,n})$ and $\sum_n Z_{1,n} \sim \mathrm{Pois}(\sum_n \lambda_{1,n})$ due to stability by convolution of the Poisson distribution, hence the result. □

**Proposition 4** (Posterior expectation of Poisson components)**.** *Let $X_s \sim \mathrm{Pois}(\lambda_s)$ for $s \in \{0,1\}$ be two independent variables and $X = X_0 - X_1$ (thus $X \sim \mathrm{Skell}(\lambda_0, \lambda_1)$). The posterior expectation of $\{X_s\}$ conditional on $X = x$ is given by:*

$$\forall s \in \{0,1\}, \ \langle X_s \mid X = x \rangle = \lambda_s \frac{P(X = x - (-1)^s)}{P(X = x)} \tag{5}$$

*where $P(X = x)$ is given by equation (2).*

*Proof.* Let us first make the proof for $X_0$.

$$\begin{aligned}
\langle X_0 \mid X = x\rangle = &\sum_{x_0=0}^{+\infty} x_0 P\left(X_0 = x_0 \mid X = x\right) \\
= &\sum_{x_0=1}^{+\infty} x_0 \frac{P\left(X_0 = x_0, X = x\right)}{P\left(X = x\right)} \\
= &\frac{1}{P\left(X = x\right)} \sum_{x_0=1}^{+\infty} x_0 P\left(X_0 = x_0\right) P\left(X_1 = x_0 - x\right) \mathbb{1}_{x \geq x_0} \\
= &\frac{1}{P\left(X = x\right)} \sum_{x_0=1}^{+\infty} x_0 e^{-\lambda_0 - \lambda_1} \frac{\lambda_0^{x_0} \lambda_1^{x_0 - x}}{x_0! \left(x_0 - x\right)!} \mathbb{1}_{x \geq x_0} \\
= &\frac{\lambda_0}{P\left(X = x\right)} \sum_{m=0}^{+\infty} e^{-\lambda_0 - \lambda_1} \frac{\lambda_0^{m} \lambda_1^{m - (x-1)}}{m! \left(m - (x-1)\right)!} \mathbb{1}_{x-1 \geq m} \\
= &\lambda_0 \frac{P\left(X = x - 1\right)}{P\left(X = x\right)}.
\end{aligned}$$

For $X_1$, just consider r.v. $-X = X_1 - X_0$, notice that

$$\langle X_1 \mid -X = -x\rangle = \langle X_1 \mid X = x\rangle,$$

and use the previously proved property:

$$\begin{aligned}
\langle X_1 \mid -X = -x\rangle &= \lambda_1 \frac{P\left(-X = -x - 1\right)}{P\left(-X = -x\right)} \\
&= \lambda_1 \frac{P\left(X = x + 1\right)}{P\left(X = x\right)}.
\end{aligned}$$

Note that this result has been proven in [1]. □

**Proposition 5** (Posterior expectation of Poisson sources)**.** *Let* $Z_{sn} \sim \mathrm{Pois}\left(\lambda_{sn}\right)$ *for* $s \in \{0, 1\}$ *and* $n = 1 \ldots N$ *all independent and let* $X = \sum_n Z_{0,n} - \sum_n Z_{1,n}$*. The posterior expectation of* $Z_{sn}$ *conditional on* $X = x$ *is given by:*

$$\langle Z_{sn} \mid X = x\rangle = \lambda_{sn} \frac{P\left(X = x - (-1)^s\right)}{P\left(X = x\right)}. \tag{6}$$

*Proof.* Given $s \in \{0,1\}$ and $n \in [\![0, N-1]\!]$:

$$\begin{aligned}
\langle Z_{sn} \mid X = x \rangle &= \sum_z z P\left(Z_{sn} = z \mid X = x\right) \\
&= \sum_z z \sum_x P\left(Z_{sn} = z, X_s = x_s \mid X = x\right) \\
&= \sum_z z \sum_{x_s} P\left(X_s = x_s \mid X = x\right) P\left(Z_{sn} = z \mid X_s = x_s\right) \\
&= \sum_{x_s} P\left(X_s = x_s \mid X = x\right) \langle Z_{sn} \mid X_s = x_s \rangle \\
&= \sum_{x_s} P\left(X_s = x_s \mid X = x\right) x_s \frac{\lambda_{sn}}{\sum_{n'} \lambda_{sn'}} \\
&= \frac{\lambda_{sn}}{\sum_{n'} \lambda_{n'}} \langle X_s \mid X = x \rangle \\
&= \frac{\lambda_{sn}}{\sum_{n'} \lambda_{sn'}} \sum_{n'} \lambda_{sn'} \frac{P\left(X = x - s\right)}{P\left(X = x\right)} \\
&= \lambda_{sn} \frac{P\left(X = x - s\right)}{P\left(X = x\right)}.
\end{aligned}$$

From line 2 to line 3, the fact that $Z_{s,n}$ is independent from $X$ given $X_s$ is used. From line 4 to line 5, one uses the well known formula of conditional posterior expectation for a sum of Poisson r.v. ($Z_n \sim \text{Pois}\left(\lambda_n\right)$ and $X = \sum_n Z_n \Rightarrow \langle Z_n \mid X = x \rangle = x \frac{\lambda_n}{\sum_{n'} \lambda_{n'}}$). Finally from line 6 to line 7, formula (5) is used. ☐

**Corollary 6** (Posterior expectation of Skellam sources)**.** *Let $Z_n \sim \text{Skell}\left(\lambda_{0,n}, \lambda_{1,n}\right)$ for $n = 1 \dots N$ independent and $X = \sum_n Z_n$. The posterior expectation of $Z_n$ conditional on $X = x$ is given by:*

$$\langle Z_n \mid X = x \rangle = \sum_{s \in \{0,1\}} \left(-1\right)^s \lambda_{s,n} \frac{P\left(X = x - \left(-1\right)^s\right)}{P\left(X = x\right)}. \tag{7}$$

*Proof.* Each $Z_n$ is the difference between two Poisson r.v. $Z_{0,n} \sim \text{Pois}\left(\lambda_{0,n}\right)$ and $Z_{1,n} \sim \text{Pois}\left(\lambda_{1,n}\right)$. Then the result follows from equation (6) and the linear nature of the expectation operator. ☐

*Remark* 7. In source separation applications, posterior expectation can be used for the estimation of the sources $Z_n$ if parameters $\lambda_{s,n}$ are known or have been estimated. It is indeed the solution that minimizes the conditional expectation of the quadratic error:

$$\arg\min_w \left\langle \left\| \{Z_n\}_{n=1 \dots N} - w \right\|_2^2 \mid X = x \right\rangle = \left\{ \langle Z_n \mid X = x \rangle \right\}_{n=1 \dots N}. \tag{8}$$

**Proposition 8** (Alternative expression for posterior expectation formulas)**.** *If $X \sim \text{Skell}\left(\lambda_0, \lambda_1\right)$, one has for $s \in \{0,1\}$:*

$$\frac{P\left(X = x - \left(-1\right)^s\right)}{P\left(X = x\right)} = \frac{\max\left(\left(-1\right)^s x, 0\right)}{\lambda_s} + \frac{\lambda_{1-s}}{|x| + 1 + \sqrt{\lambda_0 \lambda_1}\, \mathrm{R}_{|x|+1}\left(2\sqrt{\lambda_0 \lambda_1}\right)}, \tag{9}$$

*with $R_x(z)$ defined as:*

$$\mathrm{R}_x(z) = \frac{\mathrm{I}_{x+1}(z)}{\mathrm{I}_x(z)} \tag{10}$$

*and where $\mathrm{I}_a$ is the modified Bessel function of the first kind. This formula can be used in computer programs in order to avoid numerically instability when $x \geq 0$ and $\lambda_1$ is closed to 0 (or $x < 0$ and $\lambda_0$ is closed to 0). Function $R_x(z)$ can be computed using Gautschi* et al. *method [2].*

*Proof.* Modified Bessel function of the first kind respects the following property [3]:

$$\mathrm{I}_{x-1}(z) = \frac{2x}{z}\mathrm{I}_x(z) + \mathrm{I}_{x+1}(z). \tag{11}$$

By calculating $\frac{P(X=x-s)}{P(X=x)}$ whether $x \geq 1$ or $x \leq 0$ and whether $s = 0$ or $s = 1$, equations (3) and (11) gives:

$$\begin{aligned}\frac{P(X=x-s)}{P(X=x)} &= \frac{\max\left((-1)^s x, 0\right)}{\lambda_s} + \left(\frac{\lambda_0}{\lambda_1}\right)^{-\frac{(-1)^s}{2}} \frac{\mathrm{I}_{|x|+1}\left(2\sqrt{\lambda_0\lambda_1}\right)}{\mathrm{I}_{|x|}\left(2\sqrt{\lambda_0\lambda_1}\right)} \\ &= \frac{\max\left((-1)^s x, 0\right)}{\lambda_s} + \frac{2\lambda_{1-s}}{2\left(|x|+1\right) + 2\sqrt{\lambda_0\lambda_1}\frac{\mathrm{I}_{|x|+2}\left(2\sqrt{\lambda_0\lambda_1}\right)}{\mathrm{I}_{|x|+1}\left(2\sqrt{\lambda_0\lambda_1}\right)}}.\end{aligned}$$

□

*Remark* 9. With this formula, posterior expectation of each source of a skellam mixture (equation (6)) rewrites:

$$\langle Z_{s,n} \mid X = x\rangle = \lambda_{s,n}\left(\frac{\max\left((-1)^s x, 0\right)}{\bar{\lambda}_s} + \frac{\bar{\lambda}_{1-s}}{|x| + 1 + \sqrt{\bar{\lambda}_0\bar{\lambda}_1}\,\mathrm{R}_{|x|+1}\left(2\sqrt{\bar{\lambda}_0\bar{\lambda}_1}\right)}\right) \tag{12}$$

with $\forall s \in \{0,1\}$, $\bar{\lambda}_s = \sum_n \lambda_{s,n}$.

**Proposition 10** (Posterior distribution of Poisson components)**.** *Let $Z_{s,n} \sim \mathrm{Pois}(\lambda_{s,n})$ for $s \in \{0,1\}$, $n = 1\ldots N$ and let $X = \sum_n Z_{0,n} - \sum_n Z_{1,n}$. Then the distribution of $\boldsymbol{Z} = \{Z_{s,n}\}_{s,n}$ conditional on $X = x$ and given all parameters $\boldsymbol{\lambda} = \{\lambda_{s,n}\}_{s,n}$ can be expressed as:*

$$P(\boldsymbol{Z} = \boldsymbol{z} \mid X = x) = f(\boldsymbol{z}; \boldsymbol{\lambda}, x) \tag{13}$$

*where*

$$f(\boldsymbol{z}; \boldsymbol{\lambda}, x) = \mathrm{D}(\boldsymbol{\lambda}, x)\frac{\prod_{s,n}\lambda_{s,n}^{z_{s,n}}}{\prod_{s,n} z_{s,n}!}\mathbb{1}_{\left\{x = \sum_n z_{0,n} - z_{1,n}\right\}} \tag{14}$$

*where $\mathbb{1}$ is the indicator function and with*

$$\mathrm{D}(\boldsymbol{\lambda}, x) = \frac{\prod_s \left(\sum_n \lambda_{s,n}\right)^{-\max\left((-1)^s x, 0\right)}}{{}_0F_1\left(|x|+1, \prod_s\sum_n \lambda_{s,n}\right)}\Gamma\left(|x|+1\right). \tag{15}$$

*Proof.* This formula directly derives from Bayes rule:

$$P(\boldsymbol{Z} = \boldsymbol{z} \mid X = x) = \frac{P(\boldsymbol{Z})\,P(X \mid \boldsymbol{Z})}{P(X)}. \tag{16}$$

□

## 2 Skellam-SNMF and EM algorithm

We recall that we force all $(\boldsymbol{\theta}^m, \boldsymbol{\lambda}^m)$ to be pairwise equal, meaning that we can drop superscripts $m$ for parameters. Concretely, it means that $\sum_m \bar{\lambda}_{sij}^m = M\bar{\lambda}_{sij}$ and then that

$$\forall (i,j) \in \mathcal{O},\ MX_{ij} \sim \text{Skell}\left(M\bar{\lambda}_{s=0,ij}, M\bar{\lambda}_{s=1,ij}\right) \tag{17}$$

with $\bar{\lambda}_{sij} = \sum_k \theta_{si|k}\lambda_{kj}$.

### 2.1 Analytic expression of $\mathcal{L}_{\boldsymbol{X}}^{\infty}(\boldsymbol{\theta}, \boldsymbol{\lambda})$

Equations (2) and (17) give

$$\mathcal{L}_{\boldsymbol{X}}^{M}(\boldsymbol{\theta}, \boldsymbol{\lambda}) = \sum_{ij\in\mathcal{O},s} -\bar{\lambda}_{sij} + \max\left((-1)^s X_{ij}, 0\right)\ln\bar{\lambda}_{sij} + |X_{ij}|\ln M + \frac{1}{M}\sum_{ij\in\mathcal{O}} \ln\frac{{}_0F_1\left(|MX_{ij}|+1, M^2\sigma_{ij}\right)}{\Gamma\left(|MX_{ij}|+1\right)} \tag{18}$$

where $\sigma_{ij} = \bar{\lambda}_{s=0,ij}\bar{\lambda}_{s=1,ij}$. The following relationship between ${}_0F_1$ and the modified Bessel function of the first kind

$$\forall x \geq 0,\ \frac{{}_0F_1(x+1, w)}{\Gamma(x+1)} = \frac{I_x\left(2\sqrt{w}\right)}{\left(\sqrt{w}\right)^x}, \tag{19}$$

combined with the following equivalent [3]

$$\ln \mathrm{I}_x(z) \underset{x\to\infty}{\sim} -\frac{1}{2}\ln(2\pi x) + x\sqrt{1+\left(\frac{z}{x}\right)^2} + x\ln\frac{z}{x+\sqrt{x^2+z^2}} - \frac{1}{4}\ln\left(1+\left(\frac{z}{x}\right)^2\right), \tag{20}$$

gives the following asymptotic expansion:

$$\frac{1}{M}\ln\frac{{}_0F_1\left(|MX_{ij}|+1, M^2\sigma_{ij}\right)}{\Gamma\left(|MX_{ij}|+1\right)} \underset{M\to+\infty}{\sim} -|X_{ij}|\ln M + \sqrt{X_{ij}^2+4\sigma_{ij}} - |X_{ij}|\ln\frac{|X_{ij}|+\sqrt{X_{ij}^2+4\sigma_{ij}}}{2} \tag{21}$$

which yields the expected result for $\mathcal{L}_{\boldsymbol{X}}^{\infty}(\boldsymbol{\theta}, \boldsymbol{\lambda})$ as $M \to \infty$.

### 2.2 Detailed derivation of the EM algorithm

In the expectation step of the EM algorithm, one starts by expressing the log-likelihood of the complete data (observed and latent variables),

$$\begin{aligned}\ln P\left(\boldsymbol{X}, \{\boldsymbol{Z}^m\} \mid \boldsymbol{\theta}, \boldsymbol{\lambda}\right) &= \sum_{msikj}\left(Z_{sikj}^m \ln\theta_{si|k}\lambda_{kj} - \theta_{si|k}\lambda_{kj} - \ln Z_{sikj}^m!\right)\\ &\quad + \sum_{ij}\ln\mathbb{1}_{\left\{X_{ij}=\sum_{mk} Z_{s=0,ikj}^m - Z_{s=1,ikj}^m\right\}}\\ &= \sum_{msikj} Z_{sikj}^m \ln\theta_{si|k}\lambda_{kj} - M\sum_{kj}\lambda_{kj} + cst\end{aligned} \tag{22}$$

where $cst$ does not depend on $\boldsymbol{\lambda}$ nor $\boldsymbol{\theta}$. Then, conditional expectation of this function given current estimate $\left(\hat{\boldsymbol{\theta}}^{(\eta)}, \hat{\boldsymbol{\lambda}}^{(\eta)}\right)$ is computed ($\eta$ corresponds to the iteration number):

$$C(\boldsymbol{\theta}, \boldsymbol{\lambda}) = M\sum_{sikj} W_{sikj}^{(\eta)}\ln\theta_{si|k}\lambda_{kj} - M\sum_{kj}\lambda_{kj} + cst \tag{23}$$

where

$$W_{sikj}^{(\eta)} = \begin{cases} \left\langle Z_{sikj}^{m} | X_{ij}, \hat{\boldsymbol{\theta}}^{(\eta)}, \hat{\boldsymbol{\lambda}}^{(\eta)} \right\rangle & \text{if } (i,j) \in \mathcal{O} \\ \left\langle Z_{sikj}^{m} | \hat{\boldsymbol{\theta}}^{(\eta)}, \hat{\boldsymbol{\lambda}}^{(\eta)} \right\rangle & \text{if } (i,j) \notin \mathcal{O} \end{cases}. \tag{24}$$

$W_{sikj}^{(\eta)}$ can be computed due to equation (12) :

$$W_{sikj}^{(\eta)} = \hat{\theta}_{si|k}^{(\eta)} \hat{\lambda}_{kj}^{(\eta)} U_{sij}^{(\eta)} \tag{25}$$

with

$$U_{sij}^{(\eta)} = \begin{cases} \frac{\max((-1)^s M X_{ij}, 0)}{M \bar{\lambda}_{sij}^{(\eta)}} + \frac{M \bar{\lambda}_{1-s,ij}^{(\eta)}}{|MX_{ij}|+1+M\sqrt{\sigma_{ij}^{(\eta)}}\,\mathrm{R}_{|MX_{ij}|+1}\left(2M\sqrt{\sigma_{ij}^{(\eta)}}\right)} & \text{if } (i,j) \in \mathcal{O} \\ 1 & \text{if } (i,j) \notin \mathcal{O} \end{cases} \tag{26}$$

where $\bar{\lambda}_{sij}^{(\eta)} = \hat{\theta}_{si|k}^{(\eta)} \hat{\lambda}_{kj}^{(\eta)}$ and $\sigma_{ij}^{(\eta)} = \bar{\lambda}_{s=0,ij}^{(\eta)} \bar{\lambda}_{s=1,ij}^{(\eta)}$. The second step is the maximization step where

$$\frac{1}{M} C(\boldsymbol{\theta}, \boldsymbol{\lambda}) + \frac{1}{M} \sum_{m} \ln P(\boldsymbol{\theta}^m, \boldsymbol{\lambda}^m; \boldsymbol{\alpha}, \boldsymbol{\beta}) = \frac{1}{M} C(\boldsymbol{\theta}, \boldsymbol{\lambda}) + \ln P(\boldsymbol{\theta}, \boldsymbol{\lambda}; \boldsymbol{\alpha}, \boldsymbol{\beta})$$

is maximized with respect to $\boldsymbol{\theta}$ and $\boldsymbol{\lambda}$ under nonnegativity constraint and normalization constraint $\sum_{si} \theta_{si|k} = 1$. With the introduction of Lagrange multipliers for the normalization constraint, the resulting function to be maximized is the following:

$$\begin{aligned} L(\boldsymbol{\theta}, \boldsymbol{\lambda}) = & \sum_{sikj} W_{sikj}^{(\eta)} \ln \theta_{si|k} \lambda_{kj} - \sum_{kj} \lambda_{kj} + \sum_{kj} \left( \alpha_{\upsilon(k,j)} - 1 \right) \ln \lambda_{kj} - \beta_{\omega(k,j)} \lambda_{kj} \\ & + \sum_{sik} \left( \alpha_{\varphi(s,i,k)} - 1 \right) \ln \theta_{si|k} + \sum_{k} \rho_k \left( 1 - \sum_{si} \theta_{si|k} \right) \end{aligned} \tag{27}$$

where $\rho_k$ are non-zero coefficients. If all shape hyperparameters $\boldsymbol{\alpha}$ are $\geq 1$, canceling the gradient and using equation (25) yields the following update rules for the parameters ($\propto$ means "proportional to"):

$$\hat{\lambda}_{kj}^{(\eta+1)} = \frac{\hat{\lambda}_{kj}^{(\eta)} \sum_{si} U_{sij}^{(\eta)} \hat{\theta}_{si|k}^{(\eta)} + \alpha_{\upsilon(k,j)} - 1}{1 + \beta_{\omega(k,j)}}, \tag{28}$$

$$\hat{\theta}_{si|k}^{(\eta+1)} \propto \hat{\theta}_{si|k}^{(\eta)} \sum_{j} U_{sij}^{(\eta)} \hat{\lambda}_{kj}^{(\eta)} + \alpha_{\varphi(s,i,k)} - 1 \tag{29}$$

which ensure $f_{\boldsymbol{X}}^{M}\left(\boldsymbol{\theta}^{(\eta+1)}, \boldsymbol{\lambda}^{(\eta+1)}\right) \geq f_{\boldsymbol{X}}^{M}\left(\boldsymbol{\theta}^{(\eta)}, \boldsymbol{\lambda}^{(\eta)}\right)$. If $M = +\infty$, the equivalent [3]

$$R_x(z) \sim_{x \to +\infty} \frac{z}{x + \sqrt{x^2 + z^2}} = \frac{\sqrt{z^2 + x^2} - x}{z} \tag{30}$$

can be used to compute $U_{ij}^{(\eta)}$, leading to the expected formula.

In case some shape hyperameters were $< 1$, it is not assured that equations (28) and (29) remain non-negative. Besides, the parameters cannot be equal to 0 since $f_{\boldsymbol{X}}^{M}(\boldsymbol{\theta}, \boldsymbol{\lambda})$ would not be defined. A way to solve this issue would be to add the following extra constraint on the parameters

$$\boldsymbol{\theta} \geq \epsilon \text{ and } \boldsymbol{\lambda} \geq \epsilon \tag{31}$$

with $\epsilon > 0$ and to performed the maximization stage under this constraint. However there is no closed form solutions to this problem for $\boldsymbol{\theta}$ due to the normalization constraint, and we prefer, as a workaround, to simply clip if necessary the numerator equation (28) as well as the left hand side of equation (29) to a minimum value $\epsilon$. This solution, though not complying to the exact EM algorithm, always showed to be effective in practice.

# 3 Skellam-SNMF and VBEM algorithm

## 3.1 Derivation of VBEM

In the following, notations $q_{/\boldsymbol{Z}_{ij}}$, $q_{/\lambda^m_{kj}}$ and $q_{/\boldsymbol{\theta}^m_k}$ mean respectively $\left\{q_{\boldsymbol{Z}_{i'j'}}\right\}_{(i',j')\neq(i,j)}$, $\left\{q_{\lambda^{m'}_{k'j'}}\right\}_{(m',k',j')\neq(m,k,j)}$ and $\left\{q_{\boldsymbol{\theta}^{m'}_{k'}}\right\}_{m',k'\neq m,k}$, and $q_{\boldsymbol{Z}}$, $q_\lambda$ and $q_{\boldsymbol{\theta}}$ mean $\left\{q_{\boldsymbol{Z}_{ij}}\right\}_{ij}$, $\left\{q_{\lambda^m_{kj}}\right\}_{mkj}$ and $\left\{q_{\boldsymbol{\theta}^m_k}\right\}_{mk}$. We recall also that the set of parameters and hidden sources is $W = (\{\boldsymbol{Z}^m\}_m, \{\boldsymbol{\lambda}^m\}_m, \{\boldsymbol{\theta}^m\}_m)$.

**Update for $q_{\lambda^m_{kj}}$** According to the VBEM algorithm, each $q_{\lambda_{kj}}$ should be updated sequentially and its new value should be used to update the next distribution. However, we will see that in the end, $q^{(\eta+1)}_{\lambda^m_{kj}}$ only depends on $q^{(\eta)}_{\boldsymbol{Z}}$, and this is why we do not specify the iteration number of neither $q_{/\lambda^m_{kj}}$ nor $q_{\boldsymbol{\theta}}$ for the computation of expectations.

$$
\begin{aligned}
\ln q^{(\eta+1)}_{\lambda_{kj}}\left(\lambda^m_{kj}\right) &= \left\langle \ln P\left(\boldsymbol{W}, \boldsymbol{X}_{\mathcal{O}}\right)\right\rangle_{q^{(\eta)}_{\boldsymbol{Z}}, q_{/\lambda^m_{kj}}, q_{\boldsymbol{\theta}}} \\
&= \ln P\left(\lambda^m_{kj}\right) + \sum_{si} \left\langle \ln P\left(Z^m_{sikj} \mid \boldsymbol{\lambda}, \boldsymbol{\theta}\right)\right\rangle_{q^{(\eta)}_{\boldsymbol{Z}}, q_{/\lambda^m_{kj}}, q_{\boldsymbol{\theta}}} + cst \\
&= \left(\alpha_{\upsilon(k,j)} - 1\right)\ln \lambda^m_{kj} - \lambda^m_{kj}\beta_{\omega(k,j)} + \sum_{si}\left\langle Z^m_{sikj}\ln \lambda^m_{kj}\theta^m_{si|k} - \lambda^m_{kj}\theta^m_{si|k}\right\rangle_{q^{(\eta)}_{\boldsymbol{Z}}, q_{/\lambda^m_{kj}}, q_{\boldsymbol{\theta}}} + cst \\
&= \left(\sum_{si}\left\langle Z^m_{sikj}\right\rangle_{q^{(\eta)}_{\boldsymbol{Z}_{ij}}} + \alpha_{\upsilon(k,j)} - 1\right)\ln \lambda^m_{kj} - \lambda^m_{kj}\left(1 + \beta_{\omega(b)}\right) + cst
\end{aligned} \tag{32}
$$

where in each line, terms that do no depend on $\lambda^m_{kj}$ are put in $cst$. Besides, in order to get to the last line, the equality $\left\langle \sum_{si} \theta^m_{si|k}\right\rangle_{q_{\boldsymbol{\theta}}} = 1$ due to normalization constraint on $\theta^m_{si|k}$ has been used. One can then recognize that $q^{(\eta+1)}_{\lambda^m_{kj}}$ corresponds to a gamma distribution:

$$
q^{(\eta+1)}_{\lambda^m_{kj}} = \text{Gamma}\left(\hat{\alpha}^{m^{(\eta+1)}}_{kj}, \hat{\beta}^{m^{(\eta+1)}}_{kj}\right) \tag{33}
$$

with

$$
\hat{\alpha}^{m^{(\eta+1)}}_{kj} = \sum_{si}\left\langle Z^m_{sikj}\right\rangle_{q^{(\eta)}_{\boldsymbol{Z}_{ij}}} + \alpha_{\upsilon(k,j)} \tag{34}
$$

and

$$
\hat{\beta}^{m^{(\eta+1)}}_{kj} = 1 + \beta_{\omega(k,j)} \tag{35}
$$

**Update for $q_{\boldsymbol{\theta}_k^m}$** As in the previous paragraph, iteration $(\eta)$ is not specified for distributions that at the end play no role in the computation of $q_{\boldsymbol{\theta}_k^m}^{(\eta+1)}$.

$$
\begin{aligned}
\ln q_{\boldsymbol{\theta}_k^m}^{(\eta+1)}\left(\left\{\theta_{si|k}^m\right\}_{si}\right) &= \left\langle \ln P\left(\boldsymbol{W}, \boldsymbol{X}_{\mathcal{O}}\right)\right\rangle_{q_{\boldsymbol{Z}}^{(\eta)}, q_{\lambda}, q_{/\boldsymbol{\theta}_k^m}} \\
&= \ln P\left(\left\{\theta_{si|k}^m\right\}_{si}\right) + \sum_{kj} \left\langle \ln P\left(Z_{sikj}^m \mid \boldsymbol{\lambda}, \boldsymbol{\theta}\right)\right\rangle_{q_{\boldsymbol{Z}}^{(\eta)}, q_{\lambda}, q_{/\boldsymbol{\theta}_k^m}} + cst \\
&= \sum_{si} \left(\alpha_{\varphi(s,i,k)} - 1\right) \ln \theta_{si|k}^m + \sum_{sij} \left\langle Z_{sikj}^m \ln \lambda_{kj}^m \theta_{si|k}^m - \lambda_{kj}^m \theta_{si|k}^m \right\rangle_{q_{\boldsymbol{Z}}^{(\eta)}, q_{\lambda}, q_{/\boldsymbol{\theta}_k^m}} + cst \\
&= \sum_{si} \left(\alpha_{\varphi(s,i,k)} - 1\right) \ln \theta_{si|k}^m + \sum_{si} \ln \theta_{si|k}^m \sum_{j} \left\langle Z_{sikj}^m \right\rangle_{q_{\boldsymbol{Z}_{ij}}^{(\eta)}} + cst
\end{aligned} \tag{36}
$$

since $\sum_{sij} \left\langle \lambda_{kj}^m \theta_{si|k}^m \right\rangle_{q_{\lambda}, q_{/\boldsymbol{\theta}_k^m}} = \sum_j \left\langle \lambda_{kj}^m \right\rangle_{q_{\lambda}}$ and where in each line, terms that do no depend on $\left\{\theta_{si|k}^m\right\}_{si}$ are put in $cst$. One can then recognize that $q_{\boldsymbol{\theta}_k^m}^{(\eta+1)}$ corresponds to a Dirichlet distribution:

$$
q_{\boldsymbol{\theta}_k^m}^{(\eta+1)}\left(\left\{\theta_{si|k}^m\right\}_{si}\right) = \text{Dirichlet}\left(\left\{\hat{\alpha}_{sik}^{m^{(\eta+1)}}\right\}_{si}\right) \tag{37}
$$

with

$$
\hat{\alpha}_{sik}^{m^{(\eta+1)}} = \sum_j \left\langle Z_{sikj}^m \right\rangle_{q_{\boldsymbol{Z}_{ij}}^{(\eta)}} + \alpha_{\varphi(s,i,k)} \tag{38}
$$

**Update for $q_{\boldsymbol{Z}_{ij}}$** New distributions $q_{\lambda}^{(\eta+1)}$ and $q_{\boldsymbol{\theta}}^{(\eta+1)}$ are used to compute $q_{\boldsymbol{Z}_{ij}}^{(\eta+1)}$:

$$
\begin{aligned}
\ln q_{\boldsymbol{Z}_{ij}}^{(\eta+1)}\left(\left\{Z_{sikj}^m\right\}_{msk}\right) &= \left\langle \ln P\left(\boldsymbol{W}, \boldsymbol{X}_{\mathcal{O}}\right)\right\rangle_{q_{/\boldsymbol{Z}_{ij}}, q_{\lambda}^{(\eta+1)} q_{\boldsymbol{\theta}}^{(\eta+1)}} \\
&= \sum_{msk} \left\langle \ln P\left(Z_{sikj}^m \mid \boldsymbol{\lambda}, \boldsymbol{\theta}\right)\right\rangle_{q_{/\boldsymbol{Z}_{ij}}, q_{\lambda}^{(\eta+1)}, q_{\boldsymbol{\theta}}^{(\eta+1)}} + \mathbb{1}_{ij\in\mathcal{O}} \ln P\left(X_{ij} \mid \left\{Z_{sikj}^m\right\}_{msk}\right) + cst \\
&= \sum_{msk} Z_{sikj}^m \left\langle \ln \lambda_{kj}^m \theta_{si|k}^m \right\rangle_{q_{\lambda}^{(\eta+1)}, q_{\boldsymbol{\theta}}^{(\eta+1)}} - \ln\left(Z_{sikj}^m!\right) && (39) \\
&\quad + \mathbb{1}_{ij\in\mathcal{O}} \ln \mathbb{1}_{\left\{MX_{ij} = \sum_{m'k} Z_{s=0,ikj}^{m'} - \sum_{m'k} Z_{s=1,ikj}^{m'}\right\}} + cst && (40)
\end{aligned}
$$

where in each line, we put in $cst$ all terms that do not depend on any elements of $\left\{Z_{sikj}^m\right\}_{msk}$. It can be deduced then that $q_{\boldsymbol{Z}_{ij}}^{(\eta+1)}$ corresponds to either a diffnomial distribution or a product of independent Poisson distributions:

$$
q_{\boldsymbol{Z}_{ij}}^{(\eta+1)} = \begin{cases} \text{DiffNomial}\left(MX_{ij}, \left\{\bar{\ell}_{sikj}^{m^{(\eta+1)}}\right\}_{msk}\right) & \text{if } ij \in \mathcal{O}, \\ \prod_{msk} \text{Pois}\left(\bar{\ell}_{sikj}^{m^{(\eta+1)}}\right) & \text{if } ij \notin \mathcal{O} \end{cases} \tag{41}
$$

with

$$
\bar{\ell}_{sikj}^{m^{(\eta+1)}} = \exp\left\langle \ln \lambda_{kj}\right\rangle_{q_{\lambda_{kj}^m}^{(\eta+1)}} \exp\left\langle \ln \theta_{si|k}\right\rangle_{q_{\boldsymbol{\theta}_k^m}^{(\eta+1)}} \tag{42}
$$

Note that those distributions can be used to for initialization of $q_{\boldsymbol{Z}_{ij}}^{(0)}$ after having initialized $q_{\lambda_{kj}^m}^{(0)}$ and $q_{\boldsymbol{\theta}_k^m}^{(0)}$ (just replace $\eta+1$ by 0). Moreover, if initialization of $q_{\lambda_{kj}^m}^{(0)}$ and $q_{\boldsymbol{\theta}_k^m}^{(0)}$ are the same for all $m$ as we will suppose

so, we can easily prove by recurrence that $\forall \eta$, neither $\bar{\ell}^{m^{(\eta)}}_{sikj}$, $\left\langle Z^m_{sikj} \right\rangle_{q^{(\eta)}_{\boldsymbol{Z}_{ij}}}$, $q^{(\eta)}_{\lambda^m_{kj}}$ nor $q^{(\eta)}_{\boldsymbol{\theta}^m_k}$ will depend on $m$. From now on, we will then drop superscripts $m$ when it is not necessary.

**Parameters computation for $q_{\boldsymbol{Z}_{ij}}$, $q_{\lambda_{kj}}$ and $q_{\boldsymbol{\theta}_k}$** Now we know the distributions families of $q_{\boldsymbol{Z}_{ij}}$, $q_{\lambda_{kj}}$ and $q_{\boldsymbol{\theta}_k}$, it is possible to compute update rules for their parameters. Let us start with parameters $\bar{\ell}^{m^{(\eta)}}_{sikj}$ of the distribution $q^{(\eta)}_{\boldsymbol{Z}_{ij}}$ defined in equation (42):

$$\begin{aligned}\bar{\ell}^{m^{(\eta)}}_{sikj} &= \bar{\ell}^{(\eta)}_{sikj} = \exp \left\langle \ln \lambda_{kj} \right\rangle_{q^{(\eta)}_{\lambda_{kj}}} \exp \left\langle \ln \theta_{si|k} \right\rangle_{q^{(\eta)}_{\boldsymbol{\theta}_k}} \\ &= \ell^{(\eta)}_{kj} h^{(\eta)}_{sik}\end{aligned}$$

with

$$\ell^{(\eta)}_{kj} = \exp \left\langle \ln \lambda_{kj} \right\rangle_{q^{(\eta)}_{\lambda_{kj}}} = \frac{\exp \psi \left( \hat{\alpha}^{(\eta)}_{kj} \right)}{\hat{\beta}^{(\eta)}_{kj}} \tag{43}$$

and

$$h^{(\eta)}_{sik} = \exp \left\langle \ln \theta_{\tilde{c}} \right\rangle_{q^{(\eta)}_{\boldsymbol{\theta}_k}} = \frac{\exp \psi \left( \hat{\alpha}^{(\eta)}_{sik} \right)}{\exp \psi \left( \sum_{s'i'} \hat{\alpha}^{(\eta)}_{s'i'k} \right)}. \tag{44}$$

Now, due to equation (12), one can compute $\left\langle Z^m_{sikj} \right\rangle_{q^{(\eta)}_{\boldsymbol{Z}_{ij}}}$, used to update both $q_{\lambda_{kj}}$ and $q_{\boldsymbol{\theta}_k}$:

$$\left\langle Z_{sikj} \right\rangle_{q^{(\eta)}_{\boldsymbol{Z}_{ij}}} = \bar{\ell}^{(\eta)}_{sikj} U^{(\eta)}_{sij} \tag{45}$$

with

$$U^{(\eta)}_{sij} = \begin{cases} \frac{\max(sMX_{ij},0)}{M\bar{\ell}^{(\eta)}_{sij}} + \frac{M\bar{\ell}^{(\eta)}_{1-s,ij}}{|MX_{ij}|+1+M\sqrt{\sigma^{(\eta)}_{ij}}\,\mathrm{R}_{|MX_{ij}|+1}\left(2M\sqrt{\sigma^{(\eta)}_{ij}}\right)} & \text{if } ij \in \mathcal{O}, \\ 1 & \text{if } ij \notin \mathcal{O} \end{cases} \tag{46}$$

with $\bar{\ell}^{(\eta)}_{sij} = \sum_{msk} \bar{\ell}^{(\eta)}_{sikj}$ and $\sigma^{(\eta)}_{ij} = \bar{\ell}^{(\eta)}_{s=0,ij} \bar{\ell}^{(\eta)}_{s=1,ij}$. As for the EM algorithm, equation (30) can be used to compute $U^{(\eta)}_{ij}$ if $M \to \infty$. Reintegrating expressions of $\bar{\ell}^{(\eta)}_{sikj}$, $\bar{\ell}^{(\eta)}_{sij}$, $\ell^{(\eta)}_{kj}$, $h^{(\eta)}_{sik}$ and $\left\langle Z^m_{sikj} \right\rangle_{q^{(\eta)}_{\boldsymbol{Z}_{ij}}}$ in updates rules for $\hat{\alpha}^{(\eta+1)}_{jk}$ and $\hat{\alpha}^{(\eta+1)}_{sik}$ (equations (34) and (38)) gives the expected update rules.

## 3.2 Computation of ELBO

The normalized ELBO can be rewritten as:

$$g^M\left(\mathcal{Q}, \boldsymbol{X}_{\mathcal{O}}\right) = \frac{1}{M} \left\langle \ln P\left(\boldsymbol{W}, \boldsymbol{X}_{\mathcal{O}}\right) - \ln\left(\mathcal{Q}\left(\boldsymbol{W}, \boldsymbol{X}_{\mathcal{O}}\right)\right) \right\rangle_{\mathcal{Q}} \tag{47}$$

where $\mathcal{H}(\mathcal{Q}) = -\left\langle \mathcal{Q}\left(\boldsymbol{W}\right) \right\rangle_{\mathcal{Q}}$ is the entropy of distribution $\mathcal{Q}$. Expressing $\mathcal{Q}$ according to the formula given by the VBEM algorithm and decomposing

$$\ln P\left(\boldsymbol{W}, \boldsymbol{X}_{\mathcal{O}}\right) = \sum_m \ln P\left(\boldsymbol{\lambda}^m\right) + \ln P\left(\boldsymbol{\theta}^m\right) + \ln P\left(\left\{\boldsymbol{Z}^m\right\}, \boldsymbol{X}_{\mathcal{O}} \mid \left\{\boldsymbol{\lambda}^m\right\}, \left\{\boldsymbol{\theta}^m\right\}\right) \tag{48}$$

gives

$$
\begin{aligned}
g^{M}(\mathcal{Q},\boldsymbol{X}_{\mathcal{O}}) =& \sum_{mij}\left\langle \ln P\left(\left\{Z^m_{sikj}\right\}\mid \boldsymbol{\lambda},\boldsymbol{\theta}\right) - \ln q_{\boldsymbol{Z}_{ij}}\left(\left\{Z^m_{sikj}\right\}\right) + \ln P\left(X_{ij}\mid Z^m_{sikj}\right)\right\rangle_{q_{\boldsymbol{Z}_{ij}},q_{\lambda_{kj}},q_{\boldsymbol{\theta}_k}} \\
&+ \sum_{kj}\left\langle \ln P(\lambda_{kj}) - \ln q_{\lambda_{kj}}(\lambda_{kj})\right\rangle_{q_{\lambda_{kj}}} + \sum_{k}\left\langle \ln P\left(\left\{\theta_{si|k}\right\}_{si}\right) - \ln q_{\boldsymbol{\theta}_k}\left(\left\{\theta_{si|k}\right\}_{si}\right)\right\rangle_{q_{\boldsymbol{\theta}_k}} \\
=& g^M_{\boldsymbol{Z}}(\mathcal{Q},\boldsymbol{X}_{\mathcal{O}}) + \sum_{kj} g_{\lambda_{kj}}(\mathcal{Q}) + \sum_{k} g_{\boldsymbol{\theta}_k}(\mathcal{Q}).
\end{aligned} \tag{49}
$$

with

$$
\begin{aligned}
g_{\lambda_{kj}}(\mathcal{Q}) =& \left\langle \ln P(\lambda_{kj}) - \ln q_{\lambda_{kj}}(\lambda_{kj})\right\rangle_{q_{\lambda_{kj}}} \\
=& \alpha_{\upsilon(k,j)} \ln \beta_{\omega(k,j)} - \ln\Gamma\left(\alpha_{\upsilon(k,j)}\right) + \left(\alpha_{\upsilon(k,j)} - 1\right)\left(\psi(\hat{\alpha}_{kj}) - \ln\left(\hat{\beta}_{kj}\right)\right) - \beta_{\omega(k,j)}\frac{\hat{\alpha}^{(\eta)}_{kj}}{\beta^{(\eta)}_{b}} \\
&+ \hat{\alpha}_{kj} - \ln\left(\hat{\beta}_{kj}\right) + \ln\Gamma(\hat{\alpha}_{kj}) + (1-\hat{\alpha}_{kj})\,\psi(\hat{\alpha}_{kj}) \\
=& \alpha_{\upsilon(k,j)} \ln \frac{\beta_{\omega(k,j)}}{\hat{\beta}_{kj}} + \hat{\alpha}_{kj}\left(1 - \frac{\beta_{\omega(k,j)}}{\hat{\beta}_{kj}}\right) - \psi(\hat{\alpha}_{kj})\left(-\alpha_{\upsilon(k,j)}\right) - \ln\frac{\Gamma\left(\alpha_{\upsilon(k,j)}\right)}{\Gamma(\hat{\alpha}_{kj})},
\end{aligned} \tag{50}
$$

$$
\begin{aligned}
g_{\boldsymbol{\theta}_k}(\mathcal{Q}) =& \sum_{k}\left\langle \ln P\left(\left\{\theta_{si|k}\right\}_{si}\right) - \ln q_{\boldsymbol{\theta}_k}\left(\left\{\theta_{si|k}\right\}_{si}\right)\right\rangle_{q_{\boldsymbol{\theta}_k}} \\
=& -\ln\frac{\prod_{si}\Gamma\left(\alpha_{\varphi(s,i,k)}\right)}{\Gamma\left(\sum_{si}\alpha_{\varphi(s,i,k)}\right)} + \sum_{si}\left(\alpha_{\varphi(s,i,k)} - 1\right)\left(\psi(\hat{\alpha}_{sik}) - \psi\left(\sum_{s'i'}\alpha_{s'i'k}\right)\right) \\
&+ \ln\frac{\prod_{si}\Gamma(\hat{\alpha}_{sik})}{\Gamma\left(\sum_{si}\hat{\alpha}_{sik}\right)} + \psi\left(\sum_{si}\hat{\alpha}_{sik}\right)\sum_{si}\left(\alpha_{\varphi(sik)} - 1\right) - \sum_{si}\left(\hat{\alpha}_{sik} - 1\right)\psi(\hat{\alpha}_{sik}) \\
=& \ln\frac{\Gamma\left(\sum_{si}\alpha_{\varphi(s,i,k)}\right)}{\Gamma\left(\sum_{si}\hat{\alpha}_{sik}\right)} - \sum_{si}\ln\frac{\Gamma\left(\alpha_{\varphi(s,i,k)}\right)}{\Gamma(\hat{\alpha}_{sik})} - \sum_{si}\left(\hat{\alpha}_{sik} - \alpha_{\varphi(s,i,k)}\right)\left(\psi(\hat{\alpha}_{sik}) - \psi\left(\sum_{s'i'}\hat{\alpha}_{s'i'k}\right)\right),
\end{aligned} \tag{51}
$$

and

$$
\begin{aligned}
g^M_{\boldsymbol{Z}}(\mathcal{Q},\boldsymbol{X}_{\mathcal{O}}) =& \frac{1}{M}\sum_{ij}\left\langle \ln P\left(\left\{Z^m_{sikj}\right\}\mid\boldsymbol{\lambda},\boldsymbol{\theta}\right)\right\rangle_{q_{\boldsymbol{Z}_{ij}},q_{\lambda_{kj}},q_{\boldsymbol{\theta}_k}} - \left\langle \ln q_{\boldsymbol{Z}_{ij}}\left(\left\{Z^m_{sikj}\right\}_{msk}\right)\right\rangle_{q_{\boldsymbol{Z}_{ij}}} \\
&+ \left\langle \mathbb{1}_{ij\in\mathcal{O}} \ln P\left(X_{ij}\mid\left\{Z^m_{sikj}\right\}_{msk}\right)\right\rangle_{q_{\boldsymbol{Z}_{ij}}}.
\end{aligned} \tag{52}
$$

All terms that compose $g^M_{\boldsymbol{Z}}$ can be computed for a given $ij$:

$$
\left\langle \ln P\left(\left\{Z^m_{sikj}\right\}_{msk}\mid\boldsymbol{\lambda},\boldsymbol{\theta}\right)\right\rangle_{q_{\boldsymbol{Z}_{ij}},q_{\lambda_{kj}},q_{\boldsymbol{\theta}_k}} = \sum_{msk}\left\langle Z^m_{sikj}\right\rangle_{q_{\boldsymbol{Z}_{ij}}}\ln \ell_{kj}h_{sik} - \left\langle \lambda_{kj}\theta_{si|k}\right\rangle_{q_{\lambda_{kj}},q_{\boldsymbol{\theta}_k}} - \left\langle \ln Z^m_{sikj}!\right\rangle_{q_{\boldsymbol{Z}_{ij}}}, \tag{53}
$$

$$
\begin{aligned}
-\left\langle \ln q_{\boldsymbol{Z}_{ij}}\left(\left\{Z_{sikj}^{m}\right\}_{msk}\right)\right\rangle_{q_{\boldsymbol{Z}_{ij}},q_{\lambda_{kj}},q_{\boldsymbol{\theta}_k}} &= -\sum_{smk}\left\langle Z_{sikj}^{m}\right\rangle_{q_{\boldsymbol{Z}_{ij}}} \ln \ell_{kj} h_{sik} + \sum_{smk}\left\langle \ln Z_{sikj}^{m}!\right\rangle_{q_a} \\
&\quad - \mathbb{1}_{ij\in\mathcal{O}} \ln \frac{\prod_s \left(\sum_{mk}\bar{\ell}_{sikj}\right)^{-\max(sMX_{ij},0)}\Gamma\left(MX_{ij}+1\right)}{{}_0F_1\left(\left|MX_{ij}\right|+1,\prod_s\sum_{mk}\bar{\ell}_{sikj}\right)} \\
&\quad - \mathbb{1}_{ij\in\mathcal{O}}\left\langle \ln \mathbb{1}_{\left\{MX_{ij}=\sum_{mk}Z^{m}_{s=0,ikj}-\sum_{m'k}Z^{m}_{s=1,ikj}\right\}}\right\rangle_{q_{\boldsymbol{Z}_{ij}}} \\
&\quad + \mathbb{1}_{ij\notin\mathcal{O}}\sum_{smk}\bar{\ell}_{sikj}, \qquad (54)
\end{aligned}
$$

and

$$
\left\langle \ln P\left(X_{ij} \mid Z_{sikj}^{m}\right)\right\rangle_{q_{\boldsymbol{Z}_{ij}},q_{\lambda_{kj}},q_{\boldsymbol{\theta}_k}} = \mathbb{1}_{ij\in\mathcal{O}}\left\langle \ln \mathbb{1}_{\left\{MX_{ij}=\sum_{mk}Z^{m}_{s=0,ikj}-\sum_{mk}Z^{m}_{s=1,ikj}\right\}}\right\rangle_{q_{\boldsymbol{Z}_{ij}}}. \qquad (55)
$$

If one notices that $\sum_{msikj}\left\langle \lambda_{kj}\theta_{si|k}\right\rangle_{q_{\lambda_{kj}},q_{\boldsymbol{\theta}_k}} = M\sum_{kj}\left\langle\lambda_{kj}\right\rangle_{q_{\lambda_{kj}}} = M\sum_{kj}\frac{\hat{\alpha}_{kj}}{\hat{\beta}_{kj}}$, summing those three terms, simplifying and summing over $i, j$ gives

$$
\begin{aligned}
g_{\boldsymbol{Z}}^{M}\left(\mathcal{Q},\boldsymbol{X}_{\mathcal{O}}\right) = &-\sum_{kj}\frac{\hat{\alpha}_{kj}}{\hat{\beta}_{kj}} + \sum_{ij\in\mathcal{O}}\max\left(\left(-1\right)^{s}X_a,0\right)\ln M\bar{\ell}_{sij} + \frac{1}{M}\ln\frac{{}_0F_1\left(\left|MX_{ij}\right|+1,M^2\prod_s\bar{\ell}_{sij}\right)}{\Gamma\left(M\left|X_a\right|+1\right)} \\
&+\sum_{ij\notin\mathcal{O}}\sum_{s}\bar{\ell}_{sij}. \qquad (56)
\end{aligned}
$$

When $M \to +\infty$, the asymptotic equivalent (21) can be use in order to find the formula for $g_{\boldsymbol{Z}}^{\infty}\left(\mathcal{Q},\boldsymbol{X}_{\mathcal{O}}\right)$.

### 3.3 Hyperparameters estimation

*Proof of proposition 1 of the main article.* Partial derivatives of total normalized ELBO are given by:

$$
\frac{\partial}{\partial\alpha_a}\sum_t g^M\left(\mathcal{Q}^t,\boldsymbol{X}^t;\boldsymbol{\alpha},\boldsymbol{\beta}\right) = \sum_{t=1}^{T}\sum_{b\in\upsilon^{-1}(k,j)}\left[\ln\frac{\beta_{\omega(k,j)}}{\hat{\beta}_{kj}^{t}} + \psi\left(\hat{\alpha}_{kj}^{t}\right) - \psi\left(\alpha_a\right)\right] \qquad (57)
$$

and

$$
\frac{\partial}{\partial\beta_b}\sum_t \mathcal{E}\left(\mathcal{Q}^t,\boldsymbol{X}^t;\boldsymbol{\alpha},\boldsymbol{\beta}\right) = \sum_{t=1}^{T}\sum_{b\in\omega^{-1}(b)}\frac{\alpha_{\upsilon(b)}}{\beta_e} - \frac{\hat{\alpha}_{kj}^{t}}{\hat{\beta}_{kj}^{t}}. \qquad (58)
$$

There is no closed form solution for $\alpha_a$ and $\beta_b$ so that the gradient is null, but iteratively maximizing the total ELBO with respect to $\alpha_a$ and $\beta_b$ gives the expected update rules. □

*Proof of proposition 2 of the main article.* This algorithm follows from the application of a Majorization-Minimization algorithm [4] applied to the problem of minimizing $-\sum_t g^M\left(\mathcal{Q}^t,\boldsymbol{X}^t;\boldsymbol{\alpha},\boldsymbol{\beta}\right)$ with respect to $\alpha_a$

for $a \in \varphi(\{(i,k)\})$. To do so, the following majorization function can be used:

$$\begin{aligned}
-\sum_t g^M\left(\mathcal{Q}^t, \boldsymbol{X}^t; \boldsymbol{\alpha}, \boldsymbol{\beta}\right) =& \sum_{t,k} -\ln\Gamma\left(\sum_{si}\alpha_{\varphi(s,i,k)}\right) + \sum_{t,sik}\ln\Gamma\left(\alpha_{\varphi(\tilde{c})}\right) \\
&+ \sum_{t,sik}\alpha_{\varphi(s,i,k)}\left(\psi\left(\sum_{s'i'}\hat{\alpha}^t_{s'i'k}\right) - \psi\left(\hat{\alpha}^t_{sik}\right)\right) + cst \\
\leq& T\sum_k\left[-\ln\Gamma\left(\sum_{si}\alpha^{(\kappa)}_{\varphi(sik)}\right) - \psi\left(\sum_{si}\alpha^{(\kappa)}_{\varphi(s,i,k)}\right)\left(\sum_{si}\alpha_{\varphi(s,i,k)} - \sum_{si}\alpha^{(\kappa)}_{\varphi(s,i,k)}\right)\right] \\
&+ T\sum_{sik}\ln\Gamma\left(\alpha_{\varphi(s,i,k)}\right) + \sum_{t,sik}\alpha_{\varphi(s,i,k)}\left(\psi\left(\sum_{s'i'}\hat{\alpha}^t_{s'i'k}\right) - \psi\left(\hat{\alpha}^t_{sik}\right)\right) + cst \qquad (59)
\end{aligned}$$

where $cst$ does not depend on $\boldsymbol{\alpha}$. This upper bound is obtained due to log-convexity of $\Gamma\left(\sum_{si}\alpha_{\varphi(s,i,k)}\right)$. Canceling its gradient leads to

$$\sum_{sik\in\varphi^{-1}(a)} -\psi\left(\sum_{s'i'}\alpha^{(\kappa)}_{\varphi(s',i',k)}\right) + \left|\varphi^{-1}(a)\right|\psi\left(\alpha_a\right) - \xi^T_a = 0 \qquad (60)$$

which leads to the expected update rule. □

# References


[1] D. Karlis and I. Ntzoufras, "Distributions based on Poisson differences with applications in sports," Department of Statistics, Athens University of Economics, Tech. Rep., 2000.

[2] W. Gautschi and J. Slavik, "On the Computation of Modified Bessel Function Ratios," *Mathematics Of Computation*, vol. 32, no. 143, pp. 865–875, 1978.

[3] D. E. Amos, "Computation of Modified Bessel Functions and Their Ratios," *Mathematics Of Computation*, vol. 28, no. 125, pp. 239–251, 1974.

[4] Y. Sun, P. Babu, and D. P. Palomar, "Majorization-Minimization Algorithms in Signal Processing, Communications, and Machine Learning," *IEEE Transactions on Signal Processing*, vol. 65, no. 3, pp. 794–816, 2017.
